# Supplementary material for: Evaluation of Adjoint Methods in Photoacoustic Tomography with Under-Sampled Sensors
Source: arXiv:1806.08558 ancillary file (2018-06-22)
Supplement: Supplementary file 1 [file supplementary-material.pdf]

# Supplementary Material

Hongxiang Lin[1], Takashi Azuma[2], Mehmet Burcin Unlu[3,4,5], and Shu Takagi[1]

[1] Department of Mechanical Engineering, The University of Tokyo, Tokyo, Japan
hongxianglin@fel.t.u-tokyo.ac.jp,
[2] Center for Disease Biology and Integrative Medicine,
The University of Tokyo, Tokyo, Japan
[3] Department of Physics, Bogazici University, Istanbul, Turkey
[4] Global Station for Quantum Medical Science and Engineering, Global Institution for Collaborative Research and Education, Hokkaido University, Sapporo, Japan
[5] Department of Radiation Oncology, Stanford University School of Medicine, Stanford, CA, USA

## 1 Derivation of the Imaging Functions

Consider that photoacoustic wave excites from optical absorbers and propagates in a two-dimensional lossless homogeneous medium with a speed of sound of $c_0$. Based on the assumption of photoacoustic effect stated in [1], photoacoustic wave propagation in an entail space is governed by wave equation. The photoacoustic signals denoted by $g(\mathbf{y}, t)$ are measured in a time interval $[0, T]$ and on a continuous ring sensor array $\varGamma$. Our aim is to recover the initial pressure distribution $p_0$ in a region of interest given the photoacoustic measurements $g(\mathbf{y}, t)$ on $\varGamma \times [0, T]$.

The imaging functions derived from Time-Reversal (TR) and Back-Projection (BP) in the following are built to approximate $p_0$ in a continuous regime. TR synthesizes a reversed wavefield propagating in the cavity $\varOmega$. The continuous reversed received waveform signals $g(\mathbf{y}, T-t)$ serve as a dynamic Dirichlet boundary condition on $\varGamma$. Then the reversed wavefield $p_{TR}(\mathbf{x}, t)$ is derived from the initial boundary value problem of wave equation:

$$\begin{cases} \Box p_{TR}(\mathbf{x}, t) = 0, & \text{in } \varOmega \times (0, T), \\ p_{TR}(\mathbf{x}, 0) = 0 = \frac{\partial p_{TR}}{\partial t}(\mathbf{x}, 0), & \text{in } \varOmega, \\ p_{TR}(\mathbf{y}, t) = \chi_\varGamma(\mathbf{y}) g(\mathbf{y}, T-t), & \text{on } \varGamma \times [0, T], \end{cases} \tag{1}$$

where the box operator is denoted by $\Box = \nabla^2 - \frac{1}{c_0^2}\frac{\partial^2}{\partial t^2}$, $\nabla^2$ is the Laplace operator, and $\chi_\varGamma(\mathbf{y})$ is a characteristic function that has a value of 1 on $\varGamma$ and vanishes otherwise. Correspondingly, the Dirichlet Green's function $G_d(\mathbf{x}, t|\mathbf{x_0}, t_0)$ for Eq. 1 is given by

$$\begin{cases} \Box G_d(\mathbf{x}, t|\mathbf{x_0}, t_0) = -\delta(\mathbf{x} - \mathbf{x_0})\delta(t - t_0), & \text{in } \varOmega \times (0, T), \\ G_d(\mathbf{x}, t = t_0|\mathbf{x_0}, t_0) = 0 = \frac{\partial G_d}{\partial t}(\mathbf{x}, t = t_0|\mathbf{x_0}, t_0), & \text{in } \varOmega, \\ G_d(\mathbf{x}, t|\mathbf{x_0}, t_0) = 0, & \text{on } \varGamma \times [0, T]. \end{cases} \tag{2}$$

The solution of Eq. 1 at the terminal time $T$ gives the TR imaging function as follows:

$$I_{TR}(\mathbf{x}) := p_{TR}(\mathbf{x},T) = \int_0^T \int_\Gamma \frac{\partial G_d}{\partial \boldsymbol{\nu}_\mathbf{y}}(\mathbf{x},T|\mathbf{y},t) g(\mathbf{y},T-t) \mathrm{d}\sigma(\mathbf{y}) \mathrm{d}t, \quad (3)$$

where $\boldsymbol{\nu}_\mathbf{y}$ is a unit normal vector of $\mathbf{y}$ on $\Gamma$.

In this work, we consider that the circular boundary $\Gamma$ of a radius of $R$ is composed by $N$ point-like sensor elements located at $\mathbf{y}_n$ $(n = 1, 2, \cdots, N)$ with equispaced arguments. By means of the Nyström method [2] applying to the surface integration in Eq. 3, the semi-discrete TR imaging function is written as

$$I_{TR}^{<N>}(\mathbf{x}) = h_N \sum_{n=1}^{N} \int_0^T \frac{\partial G_d}{\partial \nu_\mathbf{y}}(\mathbf{x},T|\mathbf{y}=\mathbf{y}_n,t) g(\mathbf{y}_n,T-t) dt + O(h_N^2), \quad (4)$$

where $h_N = 2\pi R/N$.

The BP method is used to retransmit circular waves from the point-like sensor elements serving as reversing sources. The reversed signals $g(\mathbf{y},T-t)$ are modulated at the corresponding reversing sources. Then the back-projection wavefield $p_{BP}(\mathbf{x},t)$, propagating in an entail space, satisfies

$$\begin{cases} \Box p_{BP}(\mathbf{x},t) = \frac{1}{c_0}\frac{\mathrm{d}\delta(T-t)}{\mathrm{d}t} g(\mathbf{x},T-t)\chi_\Gamma(\mathbf{x}), & \text{in } \mathbb{R}^2 \times (0,T); \\ p_{BP}(\mathbf{x},0) = 0 = \frac{\partial p_{BP}}{\partial t}(\mathbf{x},0), & \text{in } \mathbb{R}^2. \end{cases} \quad (5)$$

The free-space Green's function in two dimension is explicitly written by

$$G_0(\mathbf{x},t|\mathbf{x_0},t_0) = \begin{cases} \frac{1}{2\pi}\left((t-t_0)^2 - \frac{|\mathbf{x}-\mathbf{x_0}|^2}{c_0^2}\right)^{-\frac{1}{2}}, & \text{when } t-t_0 > \frac{|\mathbf{x}-\mathbf{x_0}|}{c_0}; \\ 0, & \text{when } t-t_0 \le \frac{|\mathbf{x}-\mathbf{x_0}|}{c_0}. \end{cases} \quad (6)$$

Analogously, we obtain the BP imaging function that arises from the solution of Eq. 5:

$$I_{BP}(\mathbf{x}) := p_{BP}(\mathbf{x},T) = \frac{1}{c_0}\int_0^T \int_\Gamma \frac{\partial G_0}{\partial t}(\mathbf{x},T|\mathbf{y},t) g(\mathbf{y},T-t) \mathrm{d}\sigma(\mathbf{y}) \mathrm{d}t, \quad (7)$$

We also have the semi-discrete BP imaging function

$$I_{BP}^{<N>}(\mathbf{x}) = \frac{h_N}{c_0} \sum_{n=1}^{N} \int_0^T \frac{\partial G_0}{\partial t}(\mathbf{x},\tau|\mathbf{y}_n,t=T) g(\mathbf{y}_n,T-\tau) d\tau + O(h_N^2). \quad (8)$$

In [3], it turns out that Eqs. 1 and 5 are equivalent if $\Gamma$ is continuous and is lied in the far field. However, we investigate the discrete case of $\Gamma$. The analysis will be derived in the frequency domain. The Fourier transform of a time-history function $f(t)$ is defined as $\hat{f}(\omega) = \int_{-\infty}^{+\infty} f(t) e^{i\omega t} dt$ where $\omega$ is an angular frequency and the hat $\wedge$ denotes the Fourier transform. And we also have the

Parseval's identity for the relation of an inner product of a time- and a frequency-domain function $f_1(t)$ and $f_2(t)$:

$$\int_{-\infty}^{+\infty} f_1(t)\overline{f_2(t)}dt = \frac{1}{2\pi}\int_{-\infty}^{+\infty} \widehat{f}_1(\omega)\overline{\widehat{f}_2(\omega)}d\omega, \tag{9}$$

where the overline denotes complex conjugate. With Eq. 9, for the sake of analysis henceforth, we write out the frequency-domain expressions of $I_{TR}^{<N>}$ and $I_{BP}^{<N>}$:

$$I_{TR}^{<N>}(\mathbf{x}) = \frac{h_N}{2\pi}\mathbf{Re}\sum_{n=1}^{N}\left\{\int_{-\infty}^{+\infty}\frac{\partial\widehat{G}_d}{\partial\nu_{\mathbf{y}}}(\mathbf{x},\mathbf{y}_n,\omega)\overline{\widehat{g}(\mathbf{y}_n,\omega)}d\omega\right\} + O(h_N^2), \tag{10}$$

$$I_{BP}^{<N>}(\mathbf{x}) = -\frac{h_N}{2\pi c_0}\mathbf{Re}\sum_{n=1}^{N}\left\{\int_{-\infty}^{+\infty} i\omega\widehat{G}_0(\mathbf{x},\mathbf{y}_n,\omega)\overline{\widehat{g}(\mathbf{y}_n,\omega)}d\omega\right\} + O(h_N^2), \tag{11}$$

where $\mathbf{Re}$ denotes the real part of a complex value. The free-space Green's function is written as $\widehat{G}_0(\mathbf{x},\mathbf{y}_n,\omega) = \frac{i}{4}H_0^{(1)}\left(\frac{\omega}{c_0}|\mathbf{x}-\mathbf{y}_n|\right)$ where $H_0^{(1)}$ is a zeroth-order Hankel function of the first kind. Note that the real parts of the imaging functions Eqs. 10 and 11 are taken since Eqs. 4 and 7 imply that the imaging functions are real. Adding $\mathbf{Re}$ stipulates that the complex-valued imaging functions still keep real resulting from the measurement $\hat{g}(\mathbf{y}_n,\omega)$ corrupted by random error.

## 2 The Assumptions of Adjoint Methods

In the real photoacoustic tomography apparatus, the ring sensor array is composed by a limited number of point-like sensor elements rather than the continuous sensor array assumed in the mathematical derivation. Data acquisition and image quality analysis are basically carried out on a finite number of the sensor elements. Therefore, the parameters appearing in Sect. 1 should be clarified.

We assume that the measurement $\{\hat{g}(\mathbf{y}_n,\omega)\}_{n=1}^N$ is $\omega_{\max}$-bandlimited, namely, the frequency components larger than $w_{\max}$ vanish. According to the Shannon's sampling theory, the images reconstructed by adjoint methods will not aliased if $N > 2R_\Gamma\omega_{\max}$ where $R_\Gamma$ denotes a radius of the sensor array [4]. Additionally, we assume the time history of a measured dataset and the spatial variable in an imaging domain are continuously sampled in order to focus the analysis on under-sampled sensors.

Note that the measured signal in the real experiment may include some signal components arising from reflection on the opposite sensor surface. To remove them, we assume that the radius of the sensor array satisfies $R_\Gamma > 2|\mathbf{a}|$. For a general initial pressure distribution $p_0$, we require its compact support satisfies $\mathrm{dist}(\mathrm{supp}\{p_0\}) < \frac{1}{2}\mathrm{dist}(\{\mathbf{y}_n\}_{n=1}^N)$, where "dist" denotes a maximum distance of a set and "supp" a support of a function (or a nonzero-value domain of a function).

Then with the aforementioned assumptions, Xu and Wang [5] shows the relation between the Dirichlet Green's function and the free-space one with the

use of geometrical optics approximation:

$$\frac{\partial G_d}{\partial \boldsymbol{\nu_y}}(\mathbf{y},t|\mathbf{a},t') \approx 2\frac{\partial G_0}{\partial \boldsymbol{\nu_y}}(\mathbf{y},t|\mathbf{a},t'), \tag{12}$$

where $\mathbf{y} \in \mathit{\Gamma}$. Equation 12 is based on the fact that the secondary reflection on the sensor surface is negligible with assuming a suitable terminal time $T$. Indeed, under a high frequency regime, the wavefield can be decomposed by the sum of all rays perpendicular to the wavefront. Suppose that in Eq. 12, the observation point $\mathbf{y}$ sufficiently closes to the reflected boundary $\mathit{\Gamma}$. The observation at $\mathbf{y}$ comprises the two rays: one directly traveling from $\mathbf{a}$ to $\mathbf{y}$ and the other reflected by $\mathit{\Gamma}$ then going to $\mathbf{y}$. These two rays share the same free-space Green's function if $\mathbf{y}$ converges to the reflected point on $\mathit{\Gamma}$. The reasonable selection of $T$ is thereby in a way of observing the first arrival of all rays in a range of $[\min_{2|\mathbf{a}|\le R_{\partial S_N}} |\mathbf{a}-\mathbf{y}|/c_0, \max_{2|\mathbf{a}|\le R_{\partial S_N}} l_{\mathrm{ref}}(\mathbf{a},\mathbf{y})/c_0]$ where $l_{\mathrm{ref}}(\mathbf{a},\mathbf{y})$ denotes a distance of the first reflected ray from $\mathbf{a}$ to $\mathbf{y}$.

## 3 Derivation of the Imaging-Function Expansions

There is only one acoustic source located at $\mathbf{a}$ in the cavity $\mathit{\Omega}$. The sensor at $\mathbf{y}$ receiving the single-source waveform signal satisfies the frequency-domain expression:

$$\hat{g}(\mathbf{y},\omega) = -i\omega F(\omega)\widehat{G_0}(\mathbf{y},\mathbf{a},\omega), \tag{13}$$

where $F(\omega)$ is a real function of the $\omega_{\max}$-bandlimited spectrum.

We first substitute Eq. 13 into the TR and the BP imaging functions, which yields a unified imaging function for the source-sensor pair $(\mathbf{a},\mathbf{y})$ configuration:

$$I_j^{<1>}(\mathbf{x}) = \frac{h_1}{2\pi}\int_{-\infty}^{+\infty} F(\omega)\ \mathrm{Re}[K_j(\mathbf{x},\omega)]d\omega,\ j = \mathrm{TR},\ \mathrm{BP}, \tag{14}$$

where the integrands are specified as $K_{TR}(\mathbf{x},\omega) = i\omega\widehat{\frac{\partial G_d}{\partial \nu_\mathbf{y}}}(\mathbf{x},\mathbf{y},\omega)\overline{\widehat{G_0}(\mathbf{y},\mathbf{a},\omega)}$, and $K_{BP}(\mathbf{x},\omega) = \frac{\omega^2}{c_0}\widehat{G_0}(\mathbf{x},\mathbf{y},\omega)\overline{\widehat{G_0}(\mathbf{y},\mathbf{a},\omega)}$. By canceling factors, we reduce $K_{TR}$ and $K_{BP}$ to $\widetilde{K_{TR}} = -32\pi c_0^3\frac{|\mathbf{y}-\mathbf{a}|}{|\mathbf{y}|}K_{TR}$ and $\widetilde{K_{BP}} = 32\pi c_0^3 K_{BP}$, respectively, such that they share an identical main lobe. Then incorporated with Eqs. 12, 19, and 20, the integrands are further specified by the following expressions:

$$\widetilde{K_{TR}}(\mathbf{x},\omega) = -\frac{i\omega}{2}\sum_{\ell=-\infty}^{+\infty} J_\ell(d_{\mathbf{x},\mathbf{a}}^{(\omega)})H_0^{(2)}(d_{\mathbf{y},\mathbf{a}}^{(\omega)})\left(H_{\ell-1}^{(1)}(d_{\mathbf{y},\mathbf{a}}^{(\omega)}) - H_{\ell+1}^{(1)}(d_{\mathbf{y},\mathbf{a}}^{(\omega)})\right)e^{i\ell\Theta}, \tag{15}$$

$$\widetilde{K_{BP}}(\mathbf{x},\omega) = \omega^2\sum_{\ell=-\infty}^{+\infty} J_\ell(d_{\mathbf{x},\mathbf{a}}^{(\omega)})H_0^{(2)}(d_{\mathbf{y},\mathbf{a}}^{(\omega)})H_\ell^{(1)}(d_{\mathbf{y},\mathbf{a}}^{(\omega)})e^{i\ell\Theta}, \tag{16}$$

where $d_{\mathbf{x},\mathbf{a}}^{(\omega)} = \frac{\omega}{c_0}|\mathbf{x}-\mathbf{a}|$ and $d_{\mathbf{y},\mathbf{a}}^{(\omega)} = \frac{\omega}{c_0}|\mathbf{y}-\mathbf{a}|$. $\mathit{\Theta}$ is the angle corresponding to the opposite side $|\mathbf{x}-\mathbf{y}|$ of the triangle formed by the points $\mathbf{a}$, $\mathbf{x}$, and $\mathbf{y}$.

Now it suffices to formulate the expansion of imaging functions. Note that the Bessel function $J_\ell(d^{(\omega)}_{\mathbf{x},\mathbf{a}})$ is bandlimited for any index $\ell$ with a fixed $d^{(\omega)}_{\mathbf{x},\mathbf{a}}$. Indeed, Figure 1 indicates that the Bessel function can be approximately separated into two regions: an oscillating region and an fast decaying one. They are bounded by the borderline $\ell = d^{(\omega)}_{\mathbf{x},\mathbf{a}}$. Thurs, when considering a small neighborhood of the source $\mathbf{a}$, we select the terms of the indices $\ell = \pm 1, 0$ out of Eqs. 15 and 16 since the value of the lower-order Bessel functions predominates in the series. Moreover, since the imaging point $\mathbf{x}$ is observed along an axial direction, the corresponding angle $\Theta$ can be chosen as 0 or $\pi$ when $\mathbf{x}$ and $\mathbf{y}$ are on the same or the opposite side about $\mathbf{a}$. Employing Hankel's asymptotic expansion Eq. 21 (c.f. [6]), we write out the BP imaging function $I^{<1>}_{BP}$ and the discrepancy function $\Delta I^{<1>}$ between TR and BP in proportion to the integration of $\widetilde{K_{BP}}$ and $\widetilde{K_{TR}} - \widetilde{K_{BP}}$ over the angular frequency domain respectively

$$\begin{aligned} I^{<1>}_{BP}(\mathbf{x}) &\propto \int_{-\infty}^{+\infty} F(\omega)\ \mathrm{Re}[\widetilde{K_{BP}}](\mathbf{x},\omega)\mathrm{d}\omega \\ &\approx \int_{-\infty}^{+\infty} F(\omega) \left[ \frac{2\omega c_0}{\pi|\mathbf{y}-\mathbf{a}|} J_0(d^{(\omega)}_{\mathbf{x},\mathbf{a}}) + O((d^{(\omega)}_{\mathbf{x},\mathbf{a}})^3) \right] \mathrm{d}\omega. \qquad (17) \\ \Delta I^{<1>}(\mathbf{x}) &\propto \int_{-\infty}^{+\infty} F(\omega)\ \mathrm{Re}[\widetilde{K_{TR}} - \widetilde{K_{BP}}](\mathbf{x},\omega)\mathrm{d}\omega \\ &\approx e^{i\Theta} \int_{-\infty}^{+\infty} F(\omega) \left[ \frac{2c_0^2}{\pi|\mathbf{y}-\mathbf{a}|^2} J_1(d^{(\omega)}_{\mathbf{x},\mathbf{a}}) + O((d^{(\omega)}_{\mathbf{x},\mathbf{a}})^4) \right] \mathrm{d}\omega \qquad (18) \end{aligned}$$

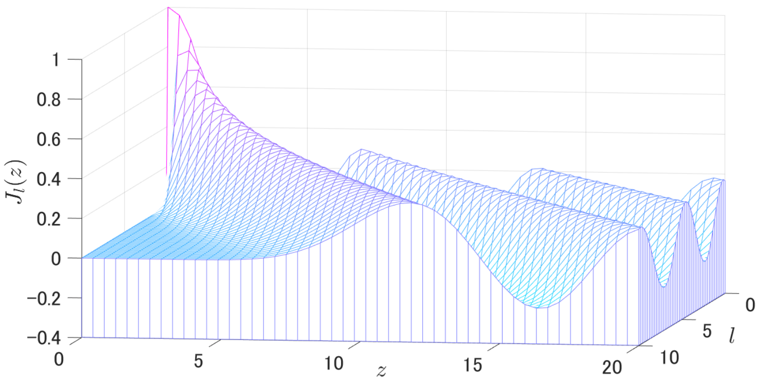


**Fig. 1.** The Bessel function $J_\ell(z)$ with respect to $\ell$ and $z$.

## Appendix: Mathematical Tools

The following formulas are related to the Bessel function $J_\ell(z)$ and the Hankel functions of the first or the second kind $H_\ell^{(j)}(z)$ ($j = 1$ or $2$) where $\ell$ is an integer and $z > 0$. They can be referred to [6] and support the derivation in Sect. 3 of the supplementary material.

1. Graf's addition theorem: If we assume $|\mathbf{x} - \mathbf{a}| < |\mathbf{y} - \mathbf{a}|$, we have

$$H_0^{(1)}\left(\frac{\omega}{c_0}|\mathbf{x}-\mathbf{y}|\right) = \sum_{\ell=-\infty}^{+\infty} J_\ell\left(\frac{\omega}{c_0}|\mathbf{x}-\mathbf{a}|\right) H_\ell^{(1)}\left(\frac{\omega}{c_0}|\mathbf{y}-\mathbf{a}|\right) e^{i\ell\Theta}, \quad (19)$$

   where $\Theta$ is the angle corresponding to the opposite side $|\mathbf{x}-\mathbf{y}|$ of the triangle formed by the points $\mathbf{a}$, $\mathbf{x}$ and $\mathbf{y}$.
2. Recurrence relation: For any integer $\ell$,

$$\frac{\mathrm{d}}{\mathrm{d}z} H_\ell^{(1)}(z) = \frac{1}{2}\left(H_{\ell-1}^{(1)}(z) - H_{\ell+1}^{(1)}(z)\right). \quad (20)$$

3. Hankel's asymptotic expansion: Define $a_0(\nu) = 1$ and

$$a_k(\nu) = \frac{(4\nu^2-1^2)(4\nu^2-3^2)\cdots(4\nu^2-(2k-1)^2)}{k!8^k}, \quad k \geq 1.$$

   Also define a function $w(\nu, z) = z - \nu\pi/2 - \pi/4$. By fixing $\nu$ and as $|z| \to \infty$, we have

$$H_\nu^{(\pm)}(z) = \left(\frac{2}{\pi z}\right)^{1/2} e^{\pm i w(\nu,z)} \left(\sum_{k=0}^{\ell-1} (-1)^k a_{2k}(\nu) z^{-2k} + O(z^{-2\ell})\right)$$
$$+ \left(\frac{2}{\pi z}\right)^{1/2} e^{\pm i(w(\nu,z)+\pi/2)} \left(\sum_{k=0}^{\ell-1} (-1)^k a_{2k+1}(\nu) z^{-2k-1} + O(z^{-2\ell-1})\right), \quad (21)$$

   where the positive (negative) sign corresponds to the Hankel function of the first (second) kind, respectively.

## References


1. Arridge, S.R., Betcke, M.M., Cox, B.T., Lucka, F., Treeby, B.E.: On the adjoint operator in photoacoustic tomography. Inverse Prob. **32**(11), 115012 (2016)
2. Kress, R.: Linear integral equations, 3rd edition. Springer-Verlag, New York (2014)
3. Ammari, H., Bretin, E., Garnier, J., Wahab, A.: Time reversal in attenuating acoustic media. Contemporary Mathematics. 548, 151-163 (2011)
4. Haltmeier, M.: Sampling conditions for the circular radon transform. IEEE Trans. Image Process. **25**(6) 2910–2919 (2016)
5. Xu, Y., Wang, L.V.: Time reversal and its application to tomography with diffracting sources. Phys. Rev. Lett. **92**(3), 033902 (2004)
6. Abramowitz, M., Stegun, I.: Handbook of mathematical functions with formulas, graphs, and mathematical tables. Dover Publications, New York (1965)
